# Supplementary material for: CC-Cert: A Probabilistic Approach to Certify General Robustness of Neural Networks
Source: arXiv:2109.10696 source file (2022-02-27)
Supplement: Supplementary file 1 [file appendix.tex]

\section*{Appendix}
\label{sec:appendix}
% \appendix

\section{Visualization of Results of Experiments.}
In this section, we provide visualisation of our experiments. %We call a model "specific" if it has lower empirical robust accuracy if trained with smoothing than if trained in a standard way, but our method catches such a behaviour and provides corresponding  probabilistic bounds.

We note that proposed metric PCA is \emph{lower bound} on a model's performance when the input is perturbed by a certain type of transform given the threshold value $\varepsilon$ for the corresponding bound. 

We verify that PCA (solid lines) are always smaller than ERA (dotted lines), which demonstrates that the proposed PCA  are increasingly tight as we increase $\varepsilon$.

% \begin{figure*}[b]
% % \centering
% % \begin{minipage}[b]{0.47\textwidth}
% \begin{subfigure}{0.47\textwidth}
% \includegraphics[width=\textwidth]{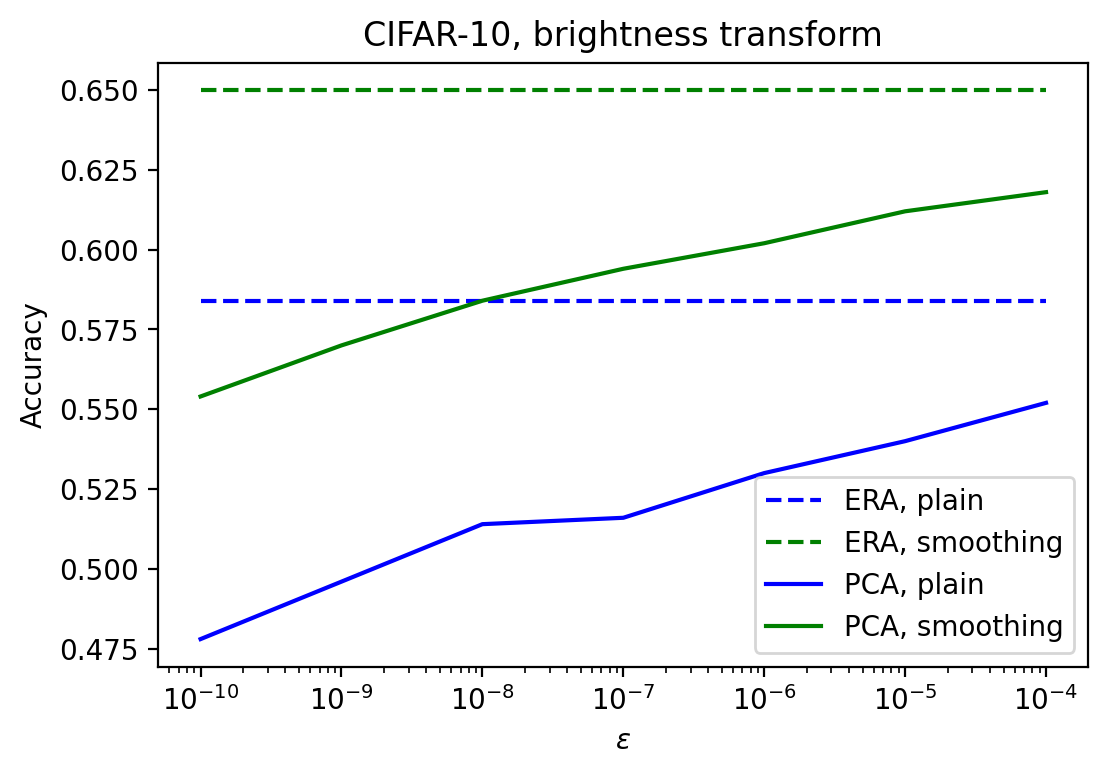}
% \caption{Experiment with brightness transform on CIFAR-10.} 
% \label{fig:cifar_brightness_exp}
% \end{subfigure}
% % \end{minipage}\hfill
% % \begin{minipage}[b]{0.47\textwidth}
% \begin{subfigure}{0.47\textwidth}
% \includegraphics[width=\textwidth]{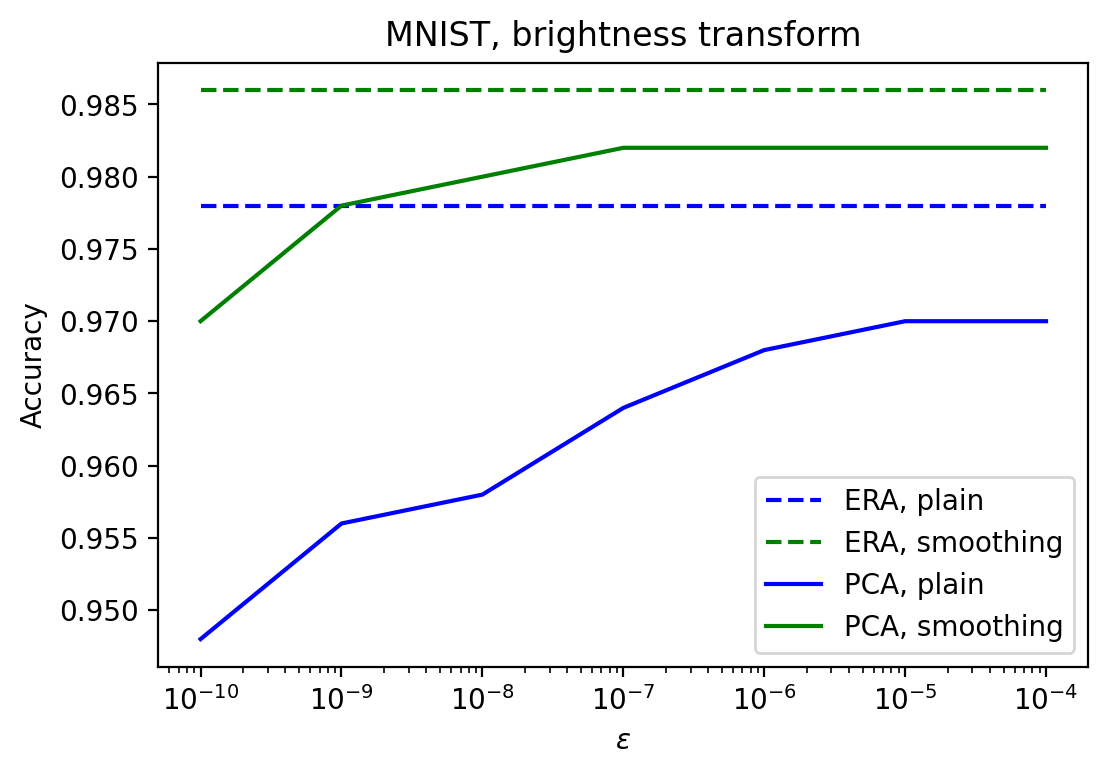}
% \caption{Experiment with brightness transform on MNIST.} 
% \label{fig:mnist_brightness_exp}
% \end{subfigure}
% % \end{minipage}
% \end{figure*}

%=====
\begin{figure}[h]
\centering
\includegraphics[width=0.48\textwidth]{figures/figures_for_appendix/CIFAR-10_brightness_transform.png}
\caption{Experiment with \emph{Brightness} on CIFAR-10.} 
\label{fig:cifar_brightness_exp}
\end{figure}

\begin{figure}[h]
\centering
\includegraphics[width=0.48\textwidth]{figures/figures_for_appendix/MNIST_brightness_transform.png}
\caption{Experiment with \emph{Brightness} on MNIST.} 
\label{fig:mnist_brightness_exp}
\end{figure}

\begin{figure}[h]
\centering
\includegraphics[width=0.48\textwidth]{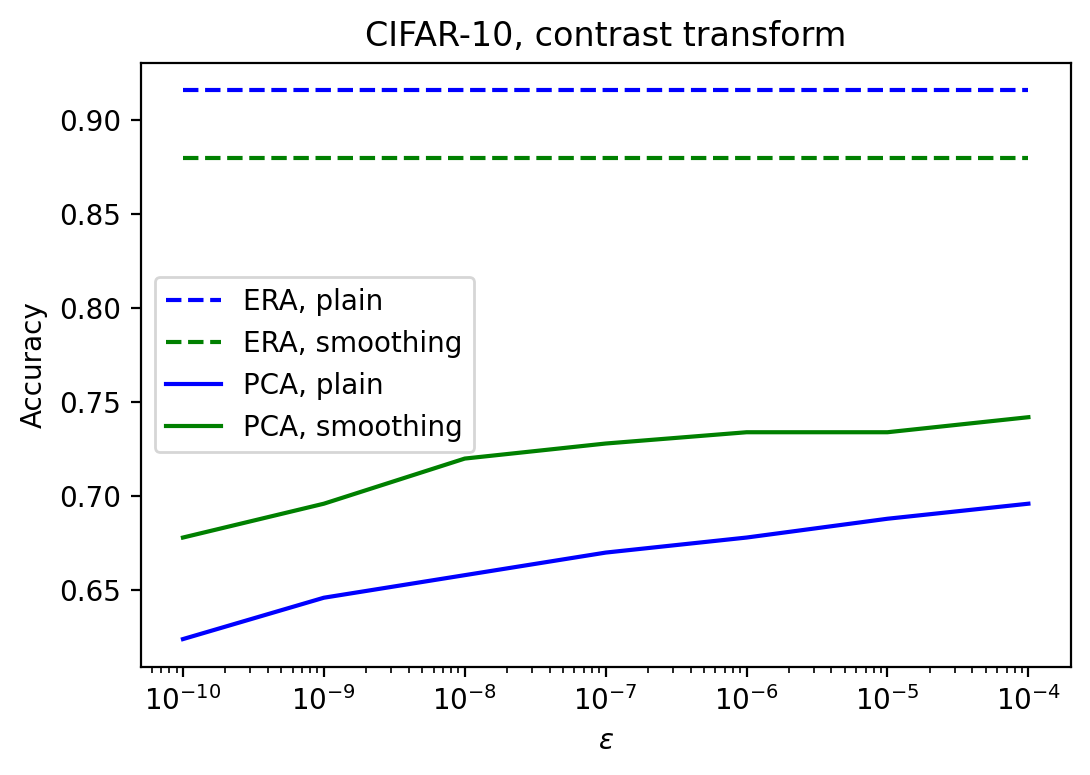}
\caption{Experiment with \emph{Contrast} on CIFAR-10.} 
\label{fig:cifar_contrast_exp}
\end{figure}

\begin{figure}[h]
\centering
\includegraphics[width=0.48\textwidth]{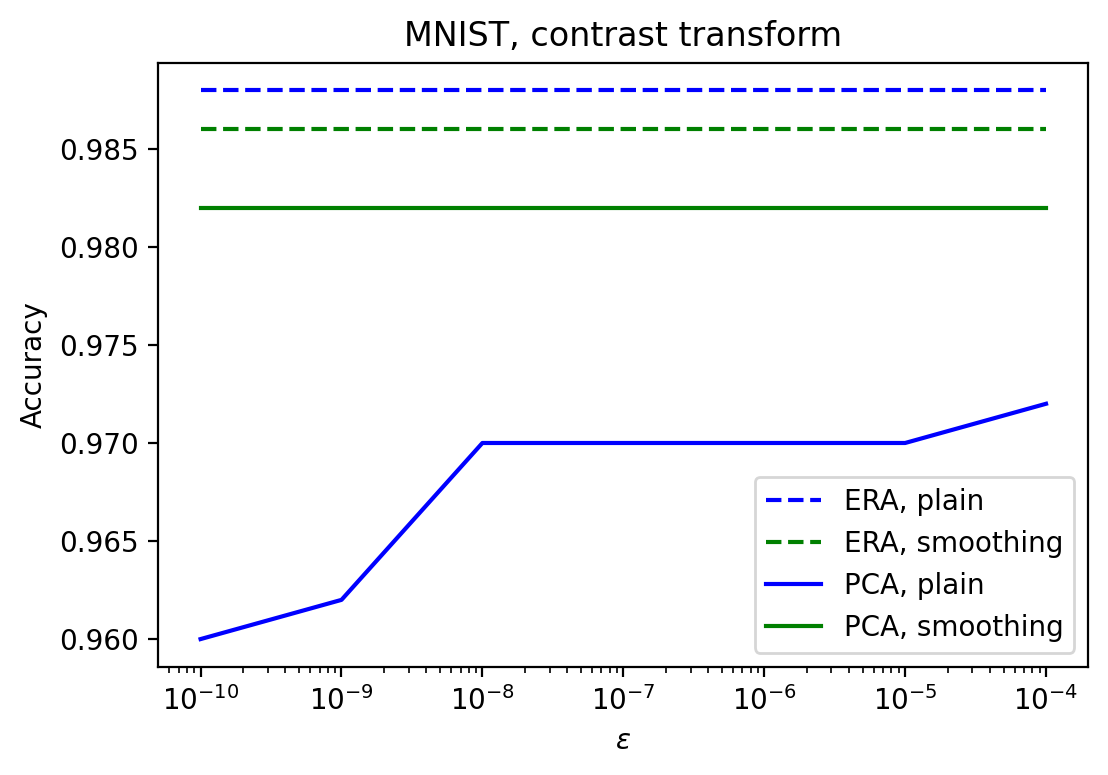}
\caption{Experiment with \emph{Contrast} on MNIST.} 
\label{fig:mnist_contrast_exp}
\end{figure}

\begin{figure}[h]
\centering
\includegraphics[width=0.48\textwidth]{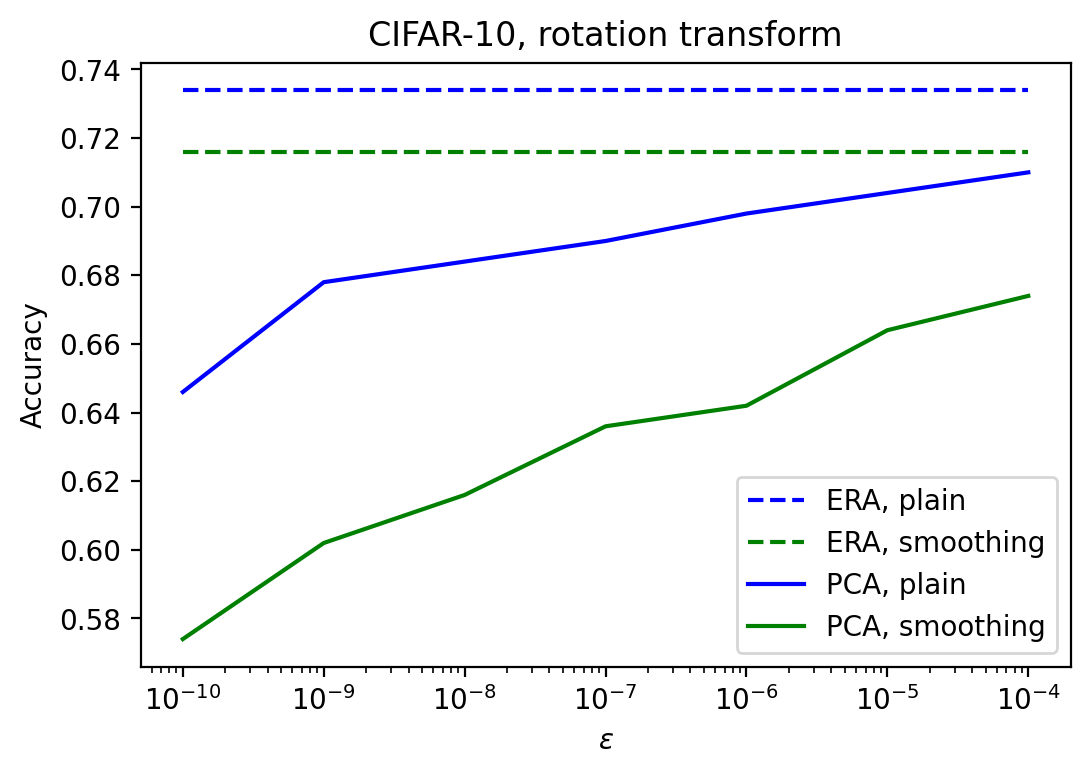}
\caption{Experiment with \emph{Rotation} on CIFAR-10.} 
\label{fig:cifar_rotation_exp}
\end{figure}

\begin{figure}[h]
\centering
\includegraphics[width=0.48\textwidth]{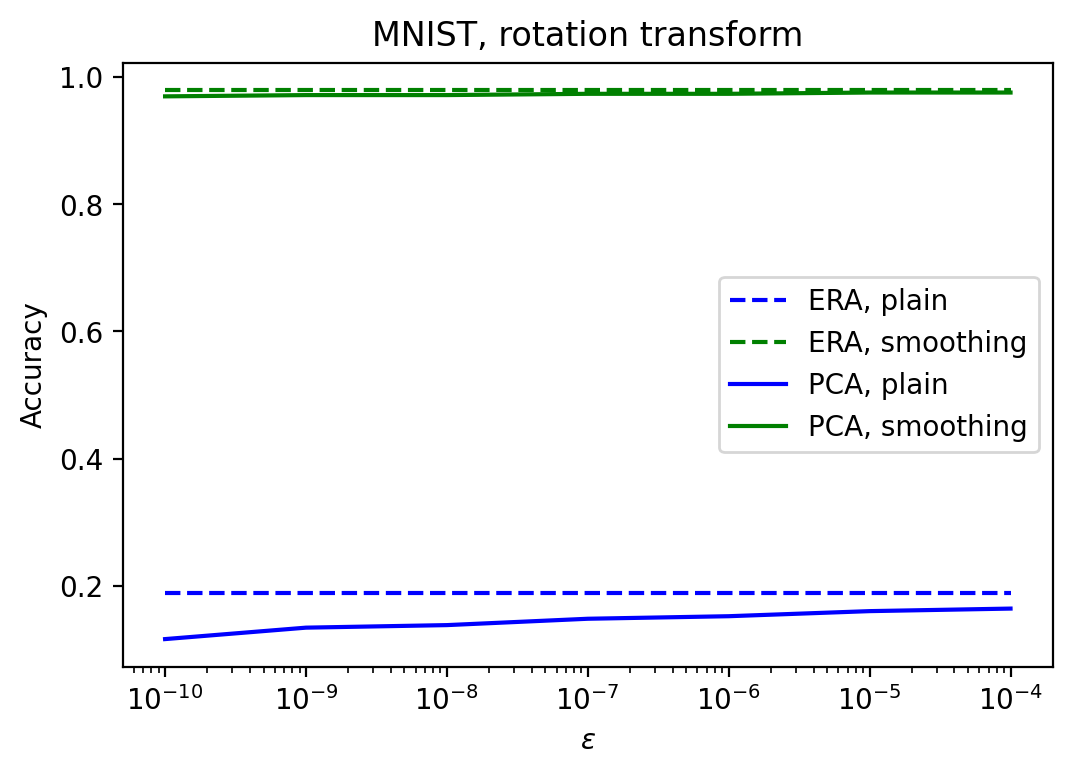}
\caption{Experiment with \emph{Rotation} on MNIST.} 
\label{fig:mnist_rotation_exp}
\end{figure}

\begin{figure}[h]
\centering
\includegraphics[width=0.48\textwidth]{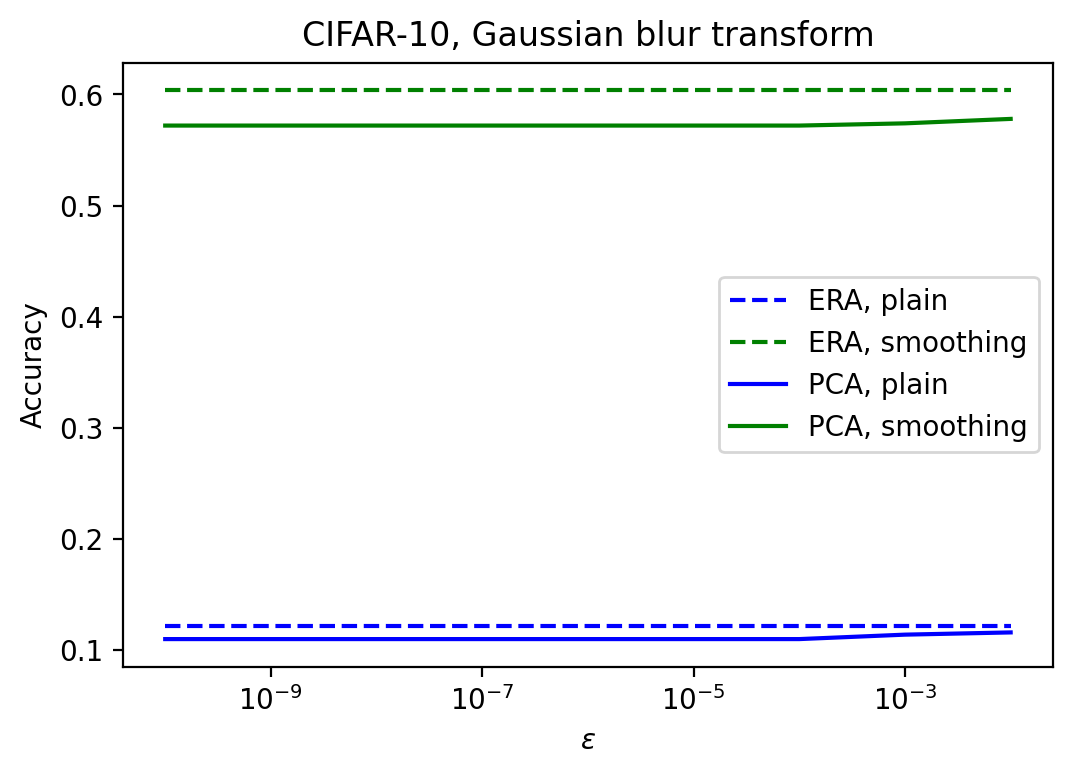}
\caption{Experiment with \emph{Gaussian blur} on CIFAR-10.} 
\label{fig:cifar_blur_exp}
\end{figure}

\begin{figure}[h]
\centering
\includegraphics[width=0.48\textwidth]{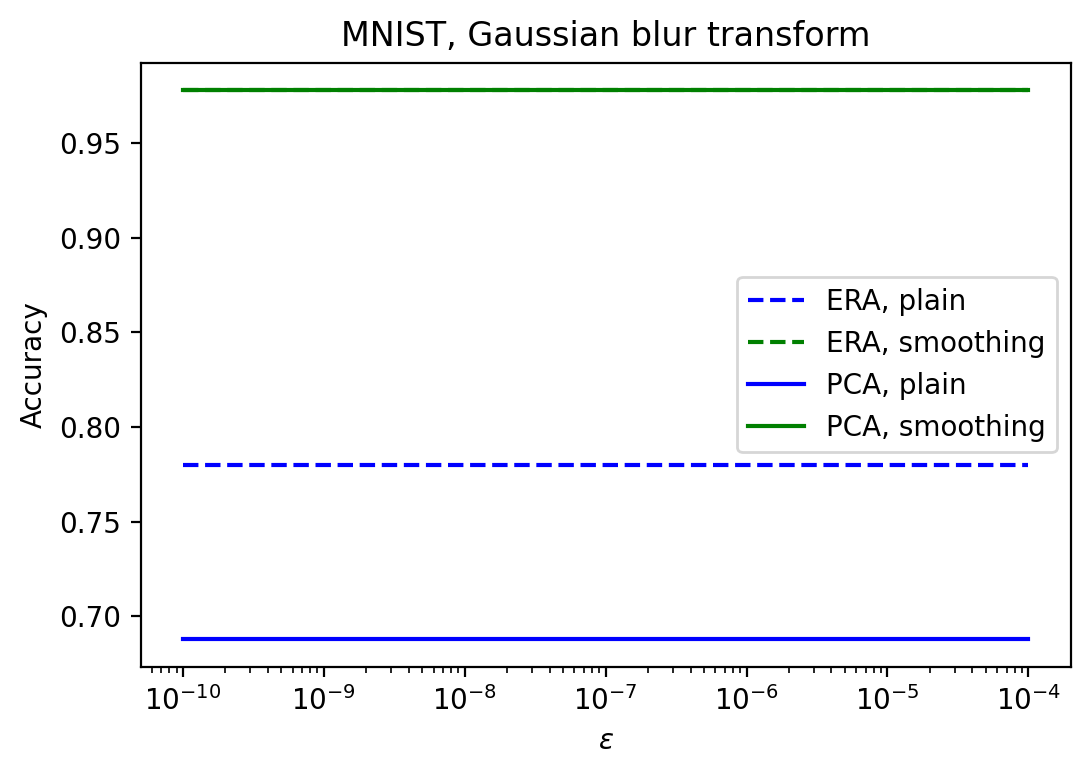}
\caption{Experiment with \emph{Gaussian blur} on MNIST.} 
\label{fig:mnist_blur_exp}
\end{figure}

\begin{figure}[h]
    \centering
    \includegraphics[width=0.48\textwidth]{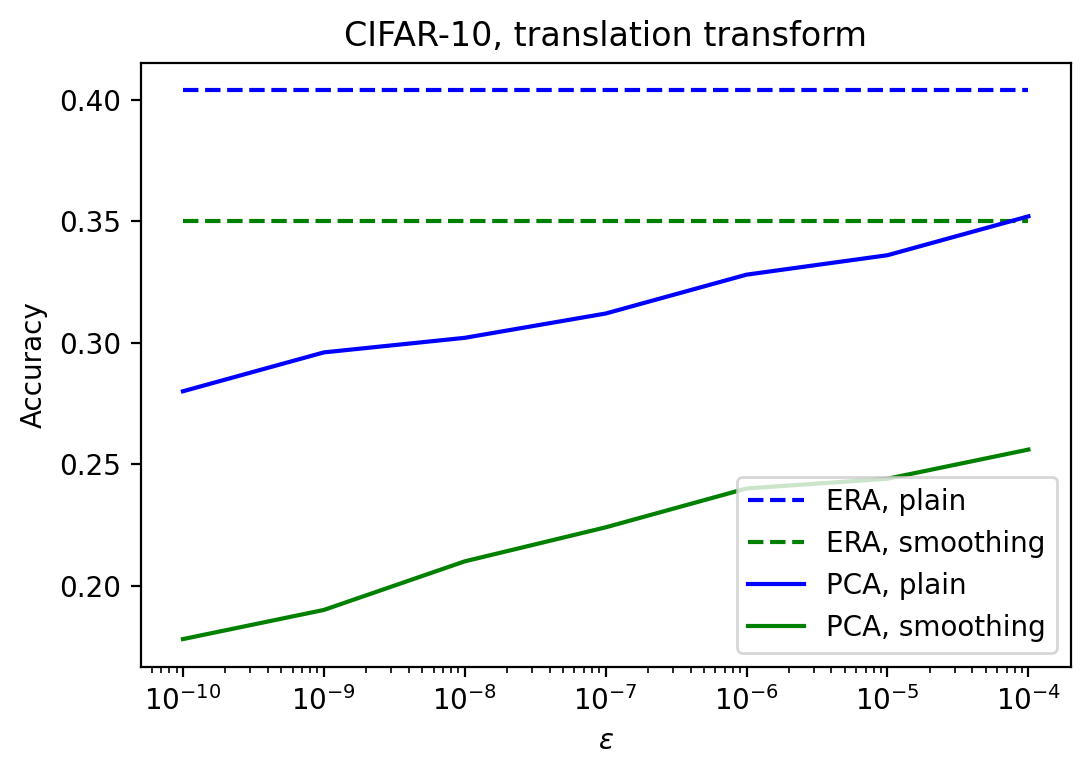}
    \caption{Experiment with \emph{Translation} on CIFAR-10.}
    \label{fig:cifar_translation_exp}
\end{figure}

\begin{figure}[h]
    \centering
    \includegraphics[width=0.48\textwidth]{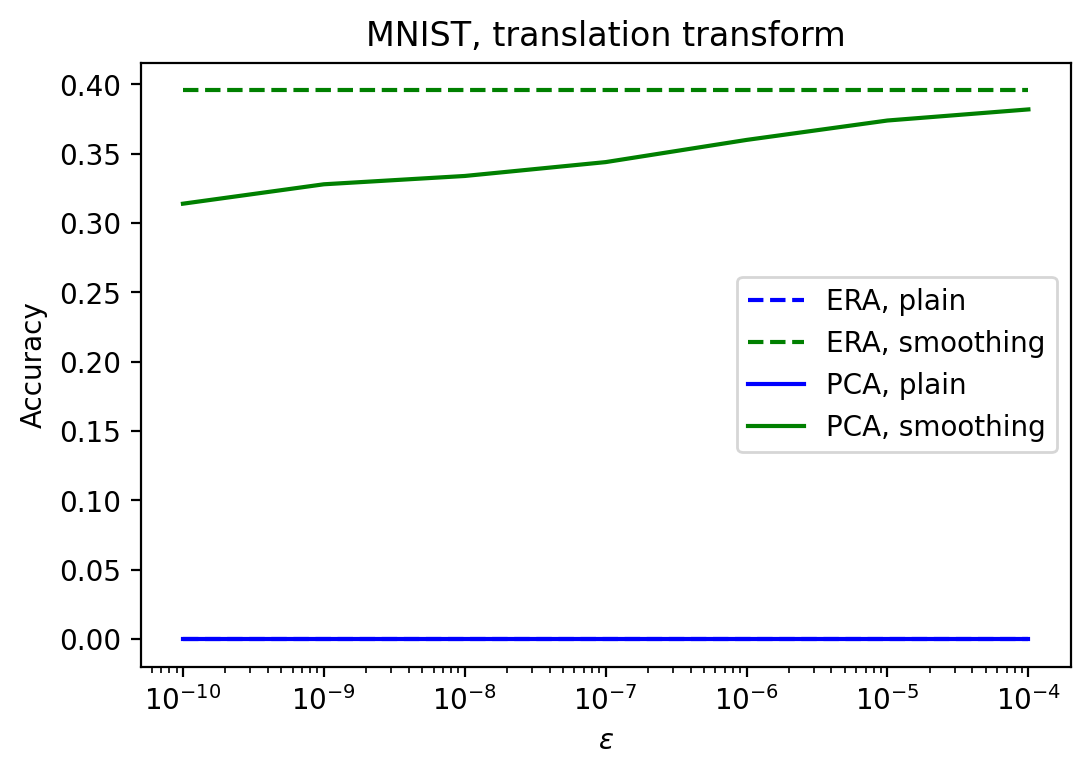}
    \caption{Experiment with \emph{Translation} on MNIST.}
    \label{fig:mnist_translation_exp}
\end{figure}

\begin{figure}[h]
    \centering
    \includegraphics[width=0.48\textwidth]{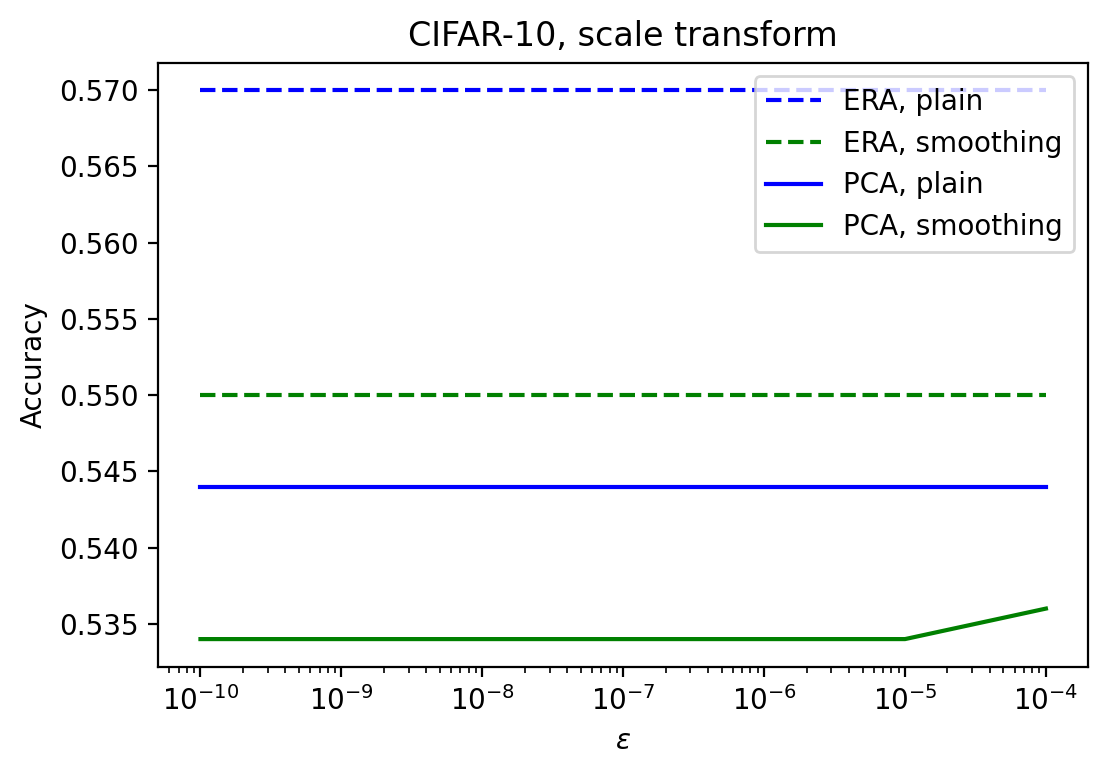}
    \caption{Experiment with \emph{Scale} on CIFAR-10.}
    \label{fig:cifar_scale_exp}
\end{figure}

\begin{figure}[h]
    \centering
    \includegraphics[width=0.48\textwidth]{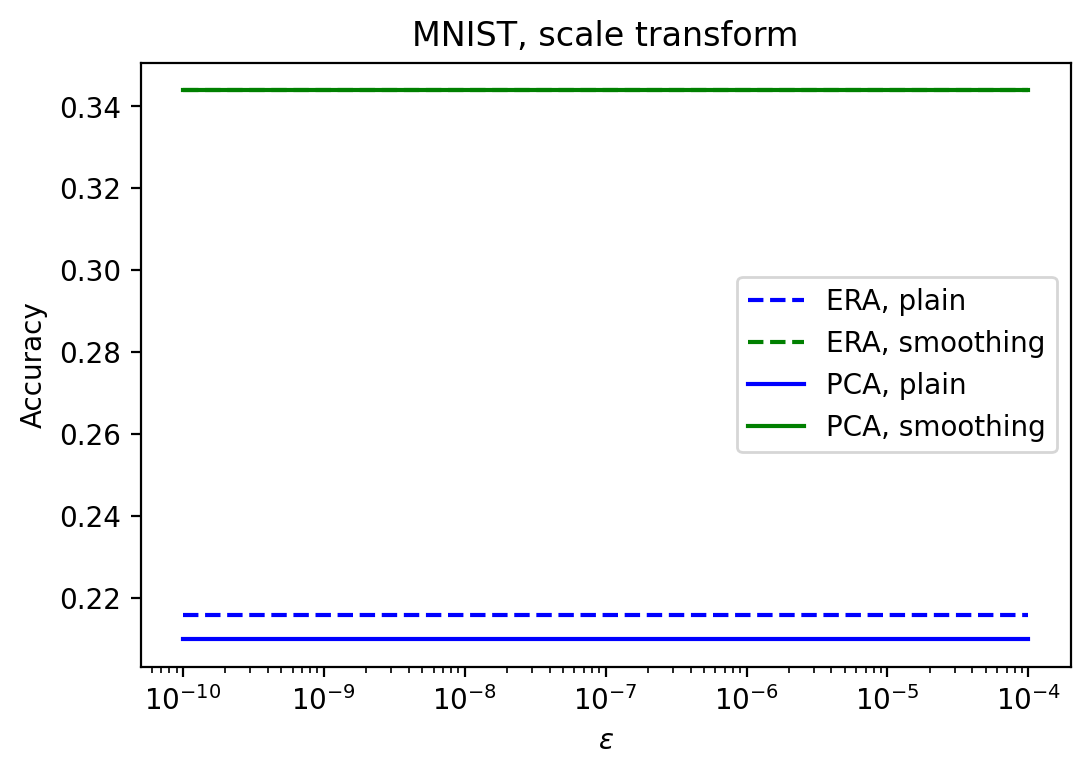}
    \caption{Experiment with \emph{Scale} on MNIST.}
    \label{fig:mnist_scale_exp}
\end{figure}

\begin{figure}[h]
    \centering
    \includegraphics[width=0.48\textwidth]{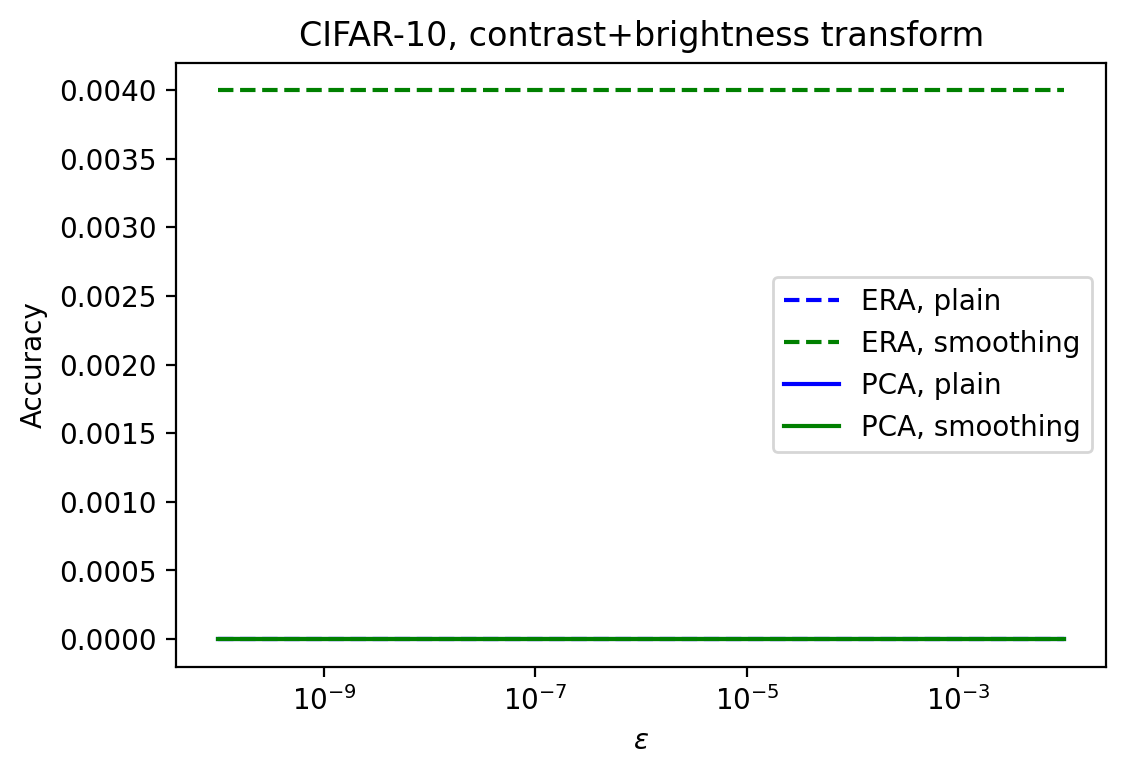}
    \caption{Experiment with \emph{Contrast and Brightness} on CIFAR-10.}
    \label{fig:cifar_contrast_brightness_exp}
\end{figure}

\begin{figure}[h]
    \centering
    \includegraphics[width=0.48\textwidth]{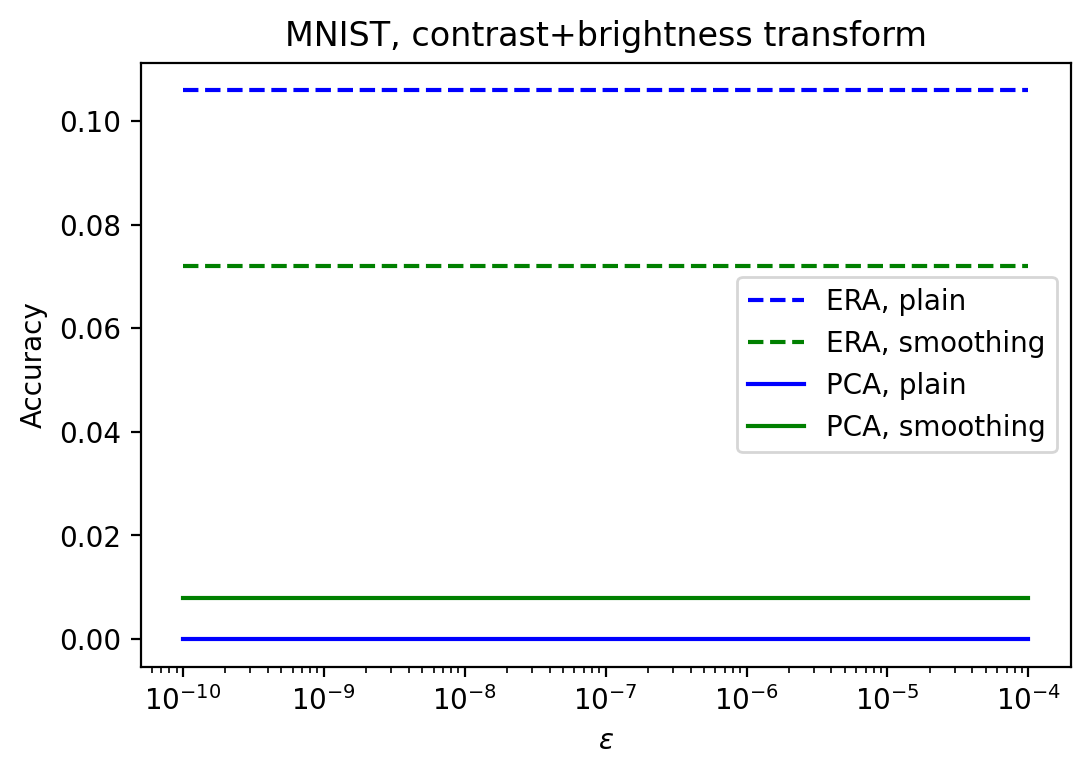}
    \caption{Experiment with \emph{Contrast and Brightness} on MNIST.}
    \label{fig:mnist_contrast_brightness_exp}
\end{figure}

\begin{figure}[h]
    \centering
    \includegraphics[width=0.48\textwidth]{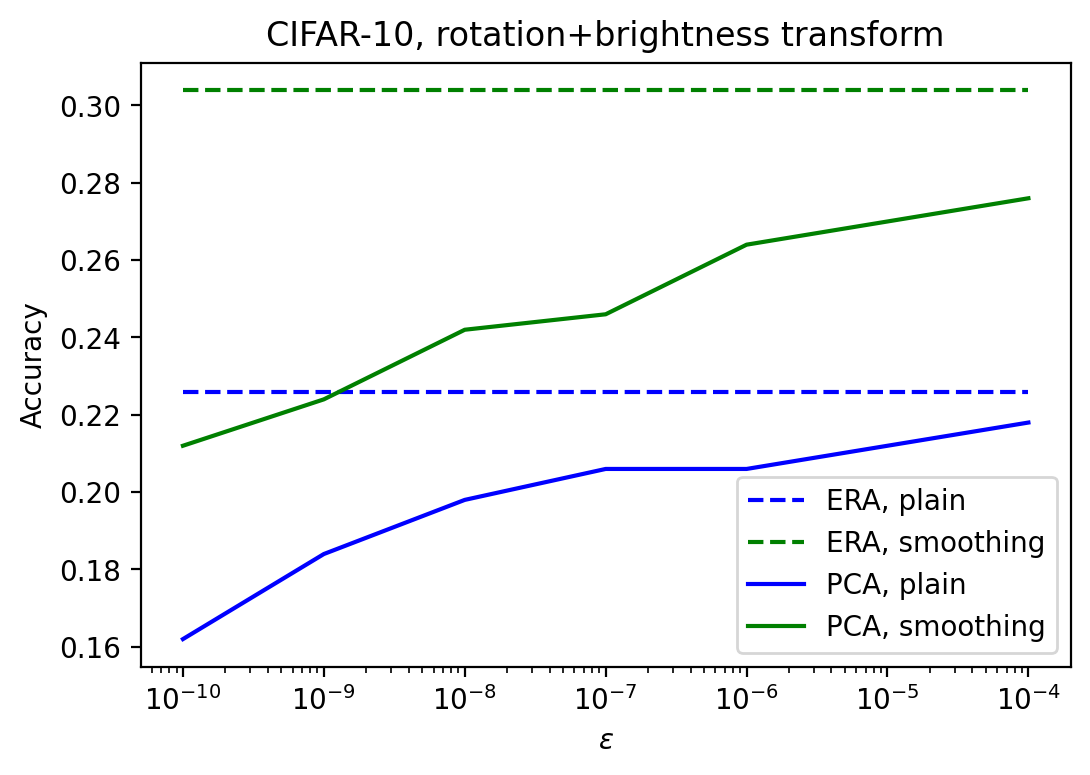}
    \caption{Experiment with \emph{Rotation and Brightness} on CIFAR-10.}
    \label{fig:cifar_rotation_brightness_exp}
\end{figure}

\begin{figure}[h]
    \centering
    \includegraphics[width=0.48\textwidth]{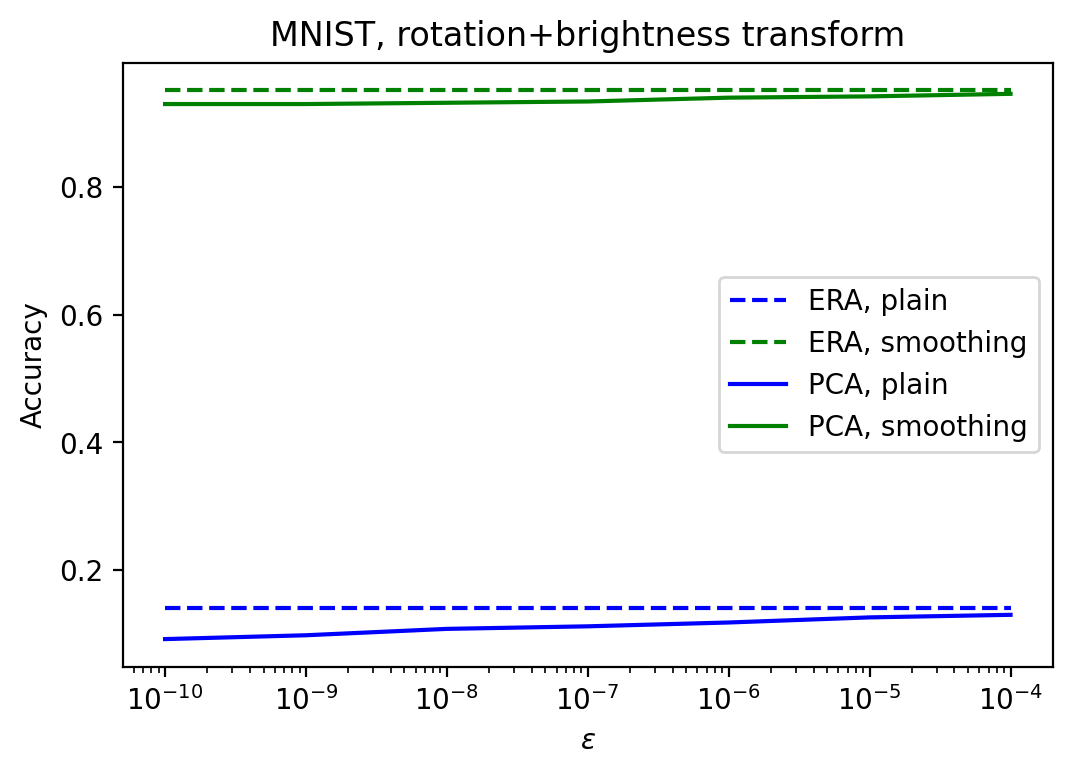}
    \caption{Experiment with \emph{Rotation and Brightness} on MNIST.}
    \label{fig:mnist_rotation_brightness_exp}
\end{figure}

\begin{figure}[h]
    \centering
    \includegraphics[width=0.48\textwidth]{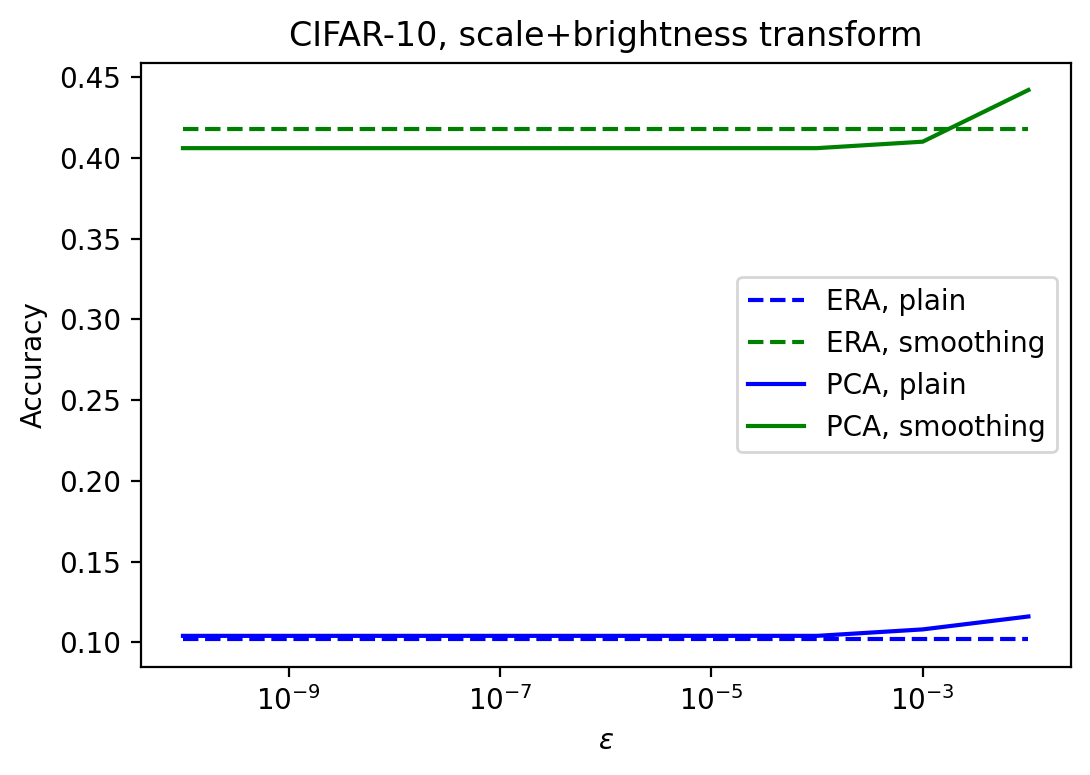}
    \caption{Experiment with \emph{Scale and Brightness} on CIFAR-10.}
    \label{fig:cifar_scale_brightness_exp}
\end{figure}

\begin{figure}[h]
    \centering
    \includegraphics[width=0.48\textwidth]{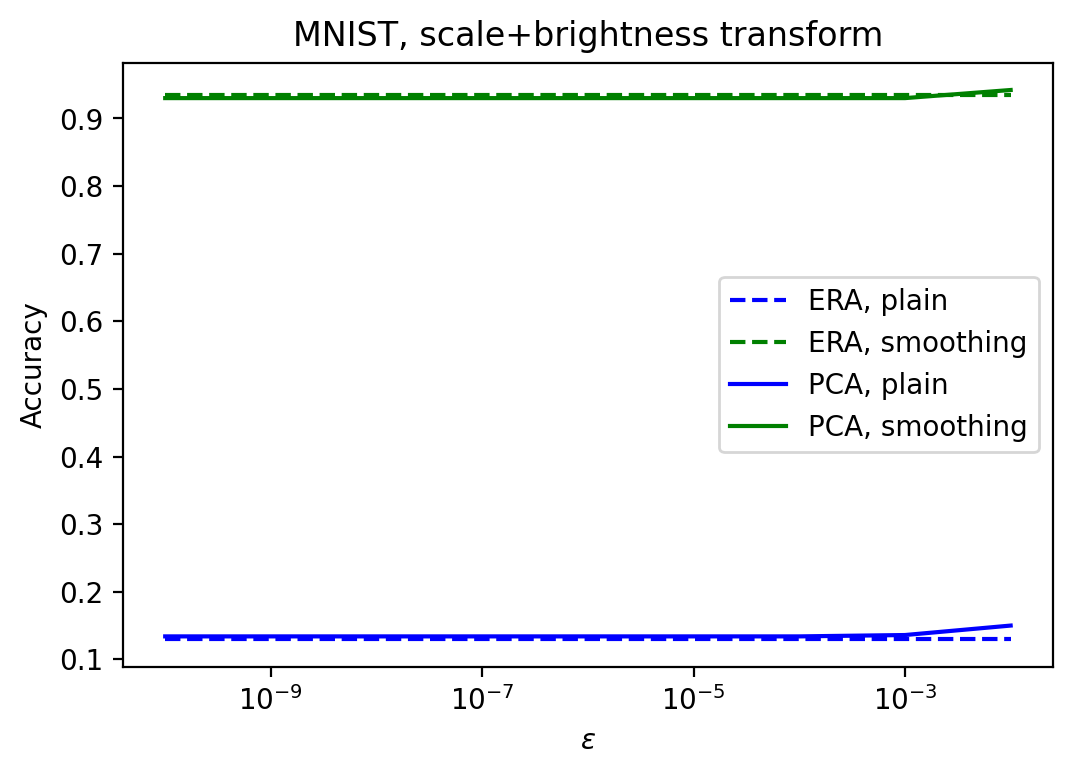}
    \caption{Experiment with \emph{Scale and Brightness} on MNIST.}
    \label{fig:mnist_scale_brightness_exp}
\end{figure}
